# Supplementary material for: Effective Anonymous Messaging: the Role of Altruism
Source: arXiv:2408.14980 source file (2024-08-27)
Supplement: Supplementary file 1 [file 7appendix.tex]

%ONLY FOR TECH REPORT VERSION!!!!! (and for future journal)
\section{Game Theory}
\label{ch:game}

\setcounter{figure}{0}  

\begin{definition}[Game]
    A normal form representation of a game is a tuple $\langle\mathcal{N},\Sigma,\mathcal{U}\rangle$, where $\mathcal{N}=\{1,\dots,m\}$ is the set of players, $\Sigma=\{S_1,\dots,S_m\}$ where $S_i=\{s_1^{(i)},s_2^{(i)},\dots\}$ is the set of actions for player $i$ and $\mathcal{U}=\{u_1,\dots,u_m\}$ is the set of payoff functions.
\end{definition}

\begin{definition}[Best Response]
    For a game $\langle\mathcal{N},\Sigma,\mathcal{U}\rangle$ the BR strategy for player $i$ for a given strategy vector $s^{(-i)}=(s^{(1)},\dots,s^{(i-1)},s^{(i+1)},\dots,s^{(m)})$ is $s_j^{(i)}$ if $\forall k\not=j: u_i(s^{(i)}_j,s^{(-i)})\geq u_i(s^{(i)}_k,s^{(-i)})$.
\end{definition}

\begin{definition}[Nash Equilibrium]
    A pure-strategy NE of a game $\langle\mathcal{N},\Sigma,\mathcal{U}\rangle$ is a strategy vector $(\hat{s}^{(1)},\dots,\hat{s}^{(m)})$ where $\hat{s}^{(i)}\in S_i$, such that for each player $i$ $\hat{s}^{(i)}$ is the best response for $\hat{s}^{(-i)}$.
\end{definition}

\begin{definition}[$\varepsilon$-Equilibrium]
    An $\varepsilon$-NE of a game $\langle\mathcal{N},\Sigma,\mathcal{U}\rangle$ is a strategy vector $(\tilde{s}^{(1)},\dots,\tilde{s}^{(m)})$ where $\tilde{s}^{(i)}\in S_i$, such that for each player $i$ the utility $U$ corresponding to the best response for $\tilde{s}^{(-i)}$ is not larger than $\frac{U}{1-\varepsilon}$.
\end{definition}

\begin{definition}[Social Optimum]
    The Social Optimum of a game $\langle\mathcal{N},\Sigma,\mathcal{U}\rangle$ is a strategy vector $(\overline{s}^{(1)},\dots,\overline{s}^{(m)})$ where $\overline{s}^{(i)}\in S_i$, such that $\max_{s_1\in S_1,\dots,s_m\in S_m}\sum_{i\in\mathcal{N}}$ $u_i(s^{(i)},\dots,s^{(i)})=\sum_{i\in\mathcal{N}}u_i(\overline{s}^{(1)},\dots,\overline{s}^{(m)})$.
\end{definition}

\begin{definition}[$\varepsilon$-Optimum]
    The $\varepsilon$-SO of a game $\langle\mathcal{N},\Sigma,\mathcal{U}\rangle$ is a strategy vector $(\overline{s}^{(1)},\dots,\overline{s}^{(m)})$ where $\overline{s}^{(i)}\in S_i$, such that for each player $i$ changing the strategy would not increase the overall utility $\hat{U}$ with larger than $\frac{\hat{U}}{1-\varepsilon}$.
\end{definition}

\begin{definition}[Price of Anarchy/Stability]
    Price of Anarchy and Stability of a game $\langle\mathcal{N},\Sigma,\mathcal{U}\rangle$ is below, where $\hat{S}$ is the set of all NEs
    $$PoA=\frac{\sum_{i\in \mathcal{N}}u_i(\overline{s}^{(1)},\dots,\overline{s}^{(m)})}{\min_{(\hat{s}^{(1)},\dots,\hat{s}^{(m)})\in\hat{S}}\sum_{i\in \mathcal{N}}u_i(\hat{s}^{(1)},\dots,\hat{s}^{(m)})}$$
    $$PoS=\frac{\sum_{i\in \mathcal{N}}u_i(\overline{s}^{(1)},\dots,\overline{s}^{(m)})}{\max_{(\hat{s}^{(1)},\dots,\hat{s}^{(m)})\in\hat{S}}\sum_{i\in \mathcal{N}}u_i(\hat{s}^{(1)},\dots,\hat{s}^{(m)})}$$ 
\end{definition}

\begin{definition}[Altruism]
    In the game $\langle\mathcal{N},\Sigma,\mathcal{U}\rangle$ player $i$ could be altruistic, if other players' utilities are also incorporated in its payoff, i.e., $u_i(\cdot)=u_i(\cdot)+\sum_{j\in N/\{i\}}\lambda_j\cdot u_j(\cdot)$ where $\lambda$ determines the nature of the altruism. 
\end{definition}

\begin{definition}[Potential Game]
    A Game $\langle\mathcal{N},\Sigma,\mathcal{U}\rangle$ is a Potential Game if there exist a potential function $\Psi$ such that $u_i(s^{(i)},s^{(-i)})-u_i(s^{(i)\prime},s^{(-i)})=\Psi(s^{(i)},s^{(-i)})-\Psi(s^{(i)\prime},s^{(-i)})$ holds for all players $i$ independently of the other player's actions.
\end{definition}

\begin{theorem}
    In every Potential Game there exists at least one NE.  
\end{theorem}

\section{FMD}
\label{ch:fmd}

FMD~\cite{beck2021fuzzy} consists of the following five probabilistic polynomial-time algorithms $(\mathsf{Setup},\mathsf{KeyGen},\mathsf{Flag},\mathsf{Extract},\mathsf{Test})$. Let us denote the set of attainable false positive rates with $\mathcal{P}$.

\begin{itemize}
    \item $\mathsf{Setup}(1^{\lambda})\xrightarrow{\$}\mathsf{pp}$. Global parameters $\mathsf{pp}$ of the FMD scheme are generated, i.e., the description of a shared cyclic group.
    \item $\mathsf{KeyGen}_{\mathsf{pp}}(1^{\lambda})\xrightarrow{\$}(pk,sk)$. This algorithm is given the global public parameters and the security parameter and outputs a public and secret key. 
    \item $\mathsf{Flag}(pk)\xrightarrow{\$}C.$ This randomized algorithm given a public key $pk$ outputs a flag ciphertext $C$.
    \item $\mathsf{Extract}(sk,p)\xrightarrow[]{}dsk$. Given a secret key $sk$ and a false positive rate $p$, the algorithm extracts a detection secret key $dsk$ iff $p\in\mathcal{P}$ or outputs $\bot$ otherwise.
    \item $\mathsf{Test}(dsk,C)\xrightarrow[]{}\{0,1\}$. The test algorithm, given a detection secret key $dsk$ and a flag ciphertext $C$, outputs a detection result.
\end{itemize}

\section{Social Graphs}
\label{ch:Data}

\begin{figure}[!b]
    \centering
    \includegraphics[width=0.5\textwidth]{graphs/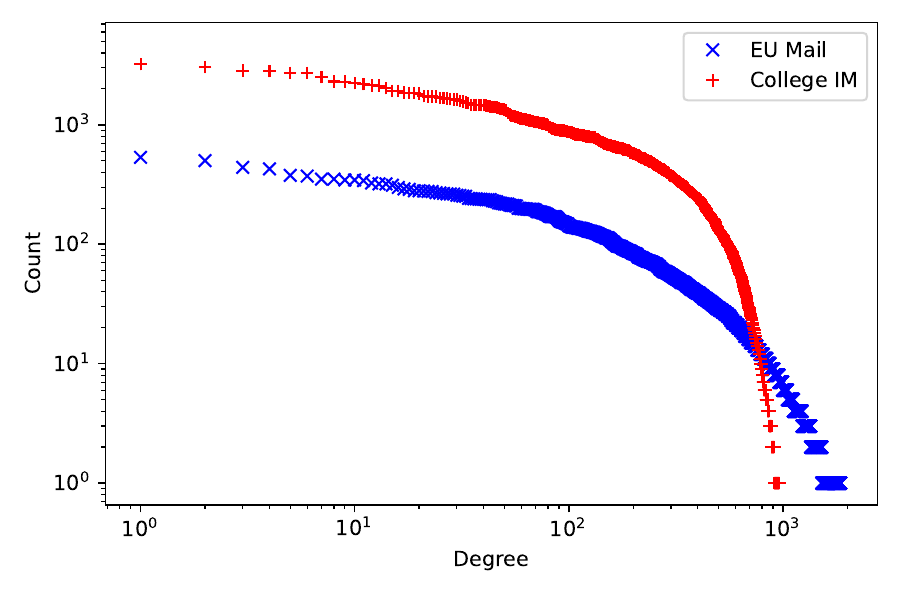}
    \caption{The distribution of messages in the "halved" graphs.}
    \label{fig:indegree_hist}
\end{figure}

\begin{figure}[!b]
    \centering
    \includegraphics[width=0.95\textwidth]{figures3/graphs_table.png}
    \caption{Comparison of various graph metrics between the College and EU datasets and their halved counterparts.}
    \label{fig:graphs_table}
\end{figure}

\newpage
\section{Results}
\label{ch:exp}

In Fig.~\ref{fig:eu_table} and~\ref{fig:college_table}, we present the results for all studied cases. \textit{Sumcost} is the overall bandwidth cost and privacy loss for every user, \textit{Iterations} is the number of steps the $\varepsilon$-BRD took before convergence, while \textit{SW \%} and \textit{iter \%} compares the costs and the running times percentage-wise where 100\% corresponds to the SW and convergence speed of the initialization achieved the highest final social welfare. The column \textit{Sum of bc at -1} and \textit{\# of top10 at -1} is the sum of normalized betweenness centrality score of users with fpr strategy $2^{-1}$ and how many of the top 10 users (according to betweenness centrality) are applying this strategy, respectively. 

%\begin{figure}[!b]
%    \centering
%    \includegraphics[width=0.9\textwidth]{figures3/cost_comparison.png}
%    \caption{Comparing the ratio of privacy and bandwidth cost to the total cost calculated. Left / right corresponds to SO and NE, blue / right corresponds to \textit{mail} and \textit{message}, even/odd column pairs correspond to 0.1 and 10. altruistic constants.}
%    \label{fig:cost_comp}
%\end{figure}

\begin{figure}[tb]
    \begin{subfigure}[b]{\textwidth}
    \centering
    \setlength{\tabcolsep}{10pt} % Column separation
    \begin{adjustbox}{max width=\textwidth}
    \begin{tabular}{|c|c|c|c|c|c|c|}
        \hline
        \textbf{Initialization strategy} & \textbf{Sumcost} & \textbf{Iterations} & \textbf{SW \%} & \textbf{Iter \%} & \textbf{sum of bc at -1} & \textbf{\# of top10 at -1} \\
        \hline
        ['bc', 'Threshold', 'all from -10'] & 1403300.0 & 133 & 100.0 & 100.0 & 0.29 & 5 \\
        \hline
        ['bc', 'Threshold', 'all from -1'] & 1405871.0 & 184 & 99.82 & 138.35 & 0.28 & 6 \\
        \hline
        ['bc', 'No Threshold', 'all from -10'] & 1408386.0 & 456 & 99.64 & 342.86 & 0.09 & 1 \\
        \hline
        ['degree', 'Threshold', 'all from -10'] & 1408377.0 & 494 & 99.64 & 371.43 & 0.09 & 1 \\
        \hline
        ['degree', 'No Threshold', 'all from -10'] & 1408314.0 & 563 & 99.64 & 423.31 & 0.09 & 1 \\
        \hline
        bc\_exp & 1452070.0 & 235 & 96.64 & 176.69 & 0.37 & 8 \\
        \hline
        random\_4 & 1453476.0 & 1597 & 96.55 & 1200.75 & 0.19 & 3 \\
        \hline
        degree\_exp & 1457898.0 & 227 & 96.26 & 170.68 & 0.23 & 2 \\
        \hline
        random\_3 & 1471467.0 & 1310 & 95.37 & 984.96 & 0.1 & 1 \\
        \hline
        bc\_lin & 1474333.0 & 1112 & 95.18 & 836.09 & 0.14 & 2 \\
        \hline
        degree\_lin & 1474379.0 & 1112 & 95.18 & 836.09 & 0.14 & 2 \\
        \hline
        ['bc', 'No Threshold', 'all from -1'] & 1474611.0 & 2295 & 95.16 & 1725.56 & 0.14 & 2 \\
        \hline
        random\_2 & 1485537.0 & 1196 & 94.46 & 899.25 & 0.12 & 2 \\
        \hline
        random\_0 & 1486204.0 & 1139 & 94.42 & 856.39 & 0.11 & 1 \\
        \hline
        random\_5 & 1487130.0 & 1150 & 94.36 & 864.66 & 0.09 & 1 \\
        \hline
        random\_1 & 1487749.0 & 995 & 94.32 & 748.12 & 0.08 & 1 \\
        \hline
        random\_6 & 1488555.0 & 1064 & 94.27 & 800.0 & 0.13 & 2 \\
        \hline
        ['degree', 'Threshold', 'all from -1'] & 1488982.0 & 2424 & 94.25 & 1822.56 & 0.09 & 1 \\
        \hline
        ['degree', 'No Threshold', 'all from -1'] & 1503379.0 & 2804 & 93.34 & 2108.27 & 0.09 & 1 \\
        \hline
  
        \end{tabular}
        \end{adjustbox}
        \caption{Global altruism with $0.1$ altruistic constant.}
        %\vspace{0.2cm}
    \end{subfigure}
    %\vspace{0.2cm}
    \begin{subfigure}[b]{\textwidth}
        \centering
        \setlength{\tabcolsep}{10pt} % Column separation
        \begin{adjustbox}{max width=\textwidth}
        \begin{tabular}{|c|c|c|c|c|c|c|}
            \hline
            \textbf{Initialization strategy} & \textbf{Sumcost} & \textbf{Iterations} & \textbf{SW \%} & \textbf{Iter \%} & \textbf{sum of bc at -1} & \textbf{\# of top10 at -1} \\
        \hline
        random\_5 & 2095436.0 & 2562 & 100.0 & 100.0 & 0.35 & 6 \\
        \hline
        random\_1 & 2099050.0 & 2800 & 99.83 & 109.29 & 0.34 & 6 \\
        \hline
        random\_2 & 2099659.0 & 2800 & 99.8 & 109.29 & 0.37 & 7 \\
        \hline
        bc\_exp & 2101048.0 & 1420 & 99.73 & 55.43 & 0.38 & 8 \\
        \hline
        random\_6 & 2101619.0 & 2759 & 99.71 & 107.69 & 0.36 & 7 \\
        \hline
        ['bc', 'Threshold', 'all from -1'] & 2103960.0 & 196 & 99.59 & 7.65 & 0.38 & 7 \\
        \hline
        random\_3 & 2103960.0 & 2654 & 99.59 & 103.59 & 0.38 & 7 \\
        \hline
        random\_4 & 2104565.0 & 2666 & 99.57 & 104.06 & 0.37 & 6 \\
        \hline
        random\_0 & 2104744.0 & 2739 & 99.56 & 106.91 & 0.37 & 7 \\
        \hline
        degree\_lin & 2105391.0 & 2433 & 99.53 & 94.96 & 0.37 & 7 \\
        \hline
        bc\_lin & 2105391.0 & 2433 & 99.53 & 94.96 & 0.37 & 7 \\
        \hline
        ['bc', 'No Threshold', 'all from -1'] & 2105391.0 & 3508 & 99.53 & 136.92 & 0.37 & 7 \\
        \hline
        ['degree', 'Threshold', 'all from -1'] & 2105391.0 & 3890 & 99.53 & 151.83 & 0.37 & 7 \\
        \hline
        ['degree', 'No Threshold', 'all from -1'] & 2105391.0 & 4582 & 99.53 & 178.84 & 0.37 & 7 \\
        \hline
        random\_7 & 2110727.0 & 2816 & 99.28 & 109.91 & 0.37 & 7 \\
        \hline
        degree\_exp & 2118458.0 & 1422 & 98.91 & 55.5 & 0.35 & 6 \\
        \hline
        ['bc', 'Threshold', 'all from -10'] & 35389817.0 & 29 & 5.92 & 1.13 & 0 & 0 \\
        \hline
        ['bc', 'No Threshold', 'all from -10'] & 35389817.0 & 352 & 5.92 & 13.74 & 0 & 0 \\
        \hline
        ['degree', 'Threshold', 'all from -10'] & 35389817.0 & 390 & 5.92 & 15.22 & 0 & 0 \\
        \hline
        ['degree', 'No Threshold', 'all from -10'] & 35389817.0 & 459 & 5.92 & 17.92 & 0 & 0 \\
        \hline
        \end{tabular}
        \end{adjustbox}
        \caption{Local altruism with $0.1$ altruism constant.}
        %\vspace{0.2cm}
    \end{subfigure}
    %\vspace{0.2cm}
    \begin{subfigure}[b]{\textwidth}
        \centering
        \setlength{\tabcolsep}{10pt} % Column separation
       \begin{adjustbox}{max width=\textwidth}
        \begin{tabular}{|c|c|c|c|c|c|c|}
            \hline
            \textbf{Initialization strategy} & \textbf{Sumcost} & \textbf{Iterations} & \textbf{SW \%} & \textbf{Iter \%} & \textbf{sum of bc at -1} & \textbf{\# of top10 at -1} \\
            \hline
            ['bc', 'Threshold', 'all from -10'] & 806635.0 & 165 & 100.0 & 100.0 & 0.35 & 6 \\
            \hline
            ['bc', 'Threshold', 'all from -1'] & 806758.0 & 144 & 99.98 & 87.27 & 0.34 & 5 \\
            \hline
            ['bc', 'No Threshold', 'all from -10'] & 816005.0 & 183 & 98.85 & 110.91 & 0.09 & 1 \\
            \hline
            ['degree', 'Threshold', 'all from -10'] & 816009.0 & 221 & 98.85 & 133.94 & 0.08 & 1 \\
            \hline
            ['degree', 'No Threshold', 'all from -10'] & 816000.0 & 290 & 98.85 & 175.76 & 0.08 & 1 \\
            \hline
            bc\_exp & 831705.0 & 412 & 96.99 & 249.7 & 0.44 & 10 \\
            \hline
            degree\_exp & 833201.0 & 389 & 96.81 & 235.76 & 0.31 & 4 \\
            \hline
            random\_3 & 833224.0 & 1788 & 96.81 & 1083.64 & 0.16 & 2 \\
            \hline
            degree\_lin & 833425.0 & 1484 & 96.79 & 899.39 & 0.15 & 2 \\
            \hline
            ['degree', 'No Threshold', 'all from -1'] & 833716.0 & 3598 & 96.75 & 2180.61 & 0.17 & 2 \\
            \hline
            random\_1 & 847292.0 & 1415 & 95.2 & 857.58 & 0.16 & 2 \\
            \hline
            random\_0 & 847606.0 & 1328 & 95.17 & 804.85 & 0.16 & 3 \\
            \hline
            random\_4 & 847602.0 & 1396 & 95.17 & 846.06 & 0.2 & 3 \\
            \hline
            random\_2 & 862640.0 & 1282 & 93.51 & 776.97 & 0.1 & 1 \\
            \hline
            bc\_lin & 862780.0 & 1020 & 93.49 & 618.18 & 0.11 & 1 \\
            \hline
            random\_5 & 862855.0 & 1215 & 93.48 & 736.36 & 0.1 & 1 \\
            \hline
            ['bc', 'No Threshold', 'all from -1'] & 863395.0 & 2203 & 93.43 & 1335.15 & 0.15 & 2 \\
            \hline
            ['degree', 'Threshold', 'all from -1'] & 863441.0 & 2511 & 93.42 & 1521.82 & 0.15 & 2 \\
            \hline
        \end{tabular}
        \end{adjustbox}
        \caption{Global altruism with $1.0$ altruism constant.}
        %\vspace{0.2cm}
    \end{subfigure}
    %\vspace{0.2cm}
    \begin{subfigure}[b]{\textwidth}
        \centering
        \setlength{\tabcolsep}{10pt} % Column separation
        \begin{adjustbox}{max width=\textwidth}
        \begin{tabular}{|c|c|c|c|c|c|c|}
            \hline
            \textbf{Initialization strategy} & \textbf{Sumcost} & \textbf{Iterations} & \textbf{SW \%} & \textbf{Iter \%} & \textbf{sum of bc at -1} & \textbf{\# of top10 at -1} \\
            \hline
            random\_8 & 820282.0 & 2677 & 100.0 & 100.0 & 0.44 & 8 \\
            \hline
            random\_3 & 820641.0 & 2726 & 99.96 & 101.83 & 0.43 & 7 \\
            \hline
            random\_1 & 820717.0 & 2682 & 99.95 & 100.19 & 0.38 & 6 \\
            \hline
            random\_2 & 820781.0 & 2785 & 99.94 & 104.03 & 0.42 & 6 \\
            \hline
            random\_4 & 820961.0 & 2697 & 99.92 & 100.75 & 0.4 & 6 \\
            \hline
            random\_0 & 820929.0 & 2718 & 99.92 & 101.53 & 0.42 & 7 \\
            \hline
            degree\_exp & 821318.0 & 1412 & 99.87 & 52.75 & 0.41 & 7 \\
            \hline
            random\_5 & 822182.0 & 2659 & 99.77 & 99.33 & 0.39 & 6 \\
            \hline
            ['degree', 'No Threshold', 'all from -10'] & 884782.0 & 579 & 92.71 & 21.63 & 0.43 & 8 \\
            \hline
            ['bc', 'Threshold', 'all from -1'] & 885172.0 & 156 & 92.67 & 5.83 & 0.42 & 7 \\
            \hline
            bc\_exp & 885243.0 & 1406 & 92.66 & 52.52 & 0.43 & 8 \\
            \hline
            degree\_lin & 886210.0 & 2417 & 92.56 & 90.29 & 0.41 & 7 \\
            \hline
            bc\_lin & 886210.0 & 2417 & 92.56 & 90.29 & 0.41 & 7 \\
            \hline
            ['bc', 'No Threshold', 'all from -1'] & 886210.0 & 3492 & 92.56 & 130.44 & 0.41 & 7 \\
            \hline
            ['degree', 'Threshold', 'all from -1'] & 886210.0 & 3880 & 92.56 & 144.94 & 0.41 & 7 \\
            \hline
            ['degree', 'No Threshold', 'all from -1'] & 886210.0 & 4574 & 92.56 & 170.86 & 0.41 & 7 \\
            \hline
            ['bc', 'No Threshold', 'all from -10'] & 887013.0 & 472 & 92.48 & 17.63 & 0.41 & 8 \\
            \hline
            ['degree', 'Threshold', 'all from -10'] & 887013.0 & 510 & 92.48 & 19.05 & 0.41 & 8 \\
            \hline
            ['bc', 'Threshold', 'all from -10'] & 33780900.0 & 27 & 2.43 & 1.01 & 0.02 & 0 \\
            \hline
        \end{tabular}
        \end{adjustbox}
        \caption{Local altruism with $1.0$ altruism constant.}
        %\vspace{0.2cm}
    \end{subfigure}
    \caption{Attributes of strategy profiles in NE reached by various initialization strategies for the \textit{mail} dataset.}
    \label{fig:eu_table}
\end{figure}

\begin{figure}[tb]
    \begin{subfigure}[b]{\textwidth}
    \centering
            \setlength{\tabcolsep}{10pt} % Column separation
        \begin{adjustbox}{max width=\textwidth}
        \begin{tabular}{|c|c|c|c|c|c|c|}
            \hline
            \textbf{Initialization strategy} & \textbf{Sumcost} & \textbf{Iterations} & \textbf{SW \%} & \textbf{Iter \%} & \textbf{sum of bc at -1} & \textbf{\# of top10 at -1} \\
            \hline
            ['bc', 'Threshold', 'all from -10'] & 215177.0 & 113 & 100.0 & 100.0 & 0.27 & 6 \\
            \hline
            ['bc', 'Threshold', 'all from -1'] & 215367.0 & 166 & 99.91 & 146.9 & 0.28 & 4 \\
            \hline
            ['degree', 'Threshold', 'all from -10'] & 250982.0 & 167 & 85.73 & 147.79 & 0.14 & 2 \\
            \hline
            ['bc', 'No Threshold', 'all from -10'] & 251019.0 & 213 & 85.72 & 188.5 & 0.14 & 2 \\
            \hline
            ['degree', 'No Threshold', 'all from -10'] & 251104.0 & 517 & 85.69 & 457.52 & 0.14 & 2 \\
            \hline
            bc\_exp & 257027.0 & 234 & 83.72 & 207.08 & 0.26 & 6 \\
            \hline
            degree\_exp & 257617.0 & 228 & 83.53 & 201.77 & 0.21 & 3 \\
            \hline
            ['degree', 'Threshold', 'all from -1'] & 263155.0 & 3006 & 81.77 & 2660.18 & 0.16 & 2 \\
            \hline
            random\_6 & 265304.0 & 2464 & 81.11 & 2180.53 & 0.11 & 1 \\
            \hline
            random\_1 & 265886.0 & 2569 & 80.93 & 2273.45 & 0.14 & 2 \\
            \hline
            ['bc', 'No Threshold', 'all from -1'] & 265864.0 & 3198 & 80.93 & 2830.09 & 0.14 & 2 \\
            \hline
            random\_4 & 268346.0 & 2236 & 80.19 & 1978.76 & 0.13 & 2 \\
            \hline
            random\_2 & 270155.0 & 2112 & 79.65 & 1869.03 & 0.07 & 1 \\
            \hline
            random\_5 & 270766.0 & 2202 & 79.47 & 1948.67 & 0.08 & 1 \\
            \hline
            random\_0 & 270871.0 & 2187 & 79.44 & 1935.4 & 0.12 & 2 \\
            \hline
            random\_3 & 270894.0 & 2261 & 79.43 & 2000.88 & 0.03 & 0 \\
            \hline
            bc\_lin & 271040.0 & 1817 & 79.39 & 1607.96 & 0.09 & 1 \\
            \hline
            ['degree', 'No Threshold', 'all from -1'] & 271040.0 & 5271 & 79.39 & 4664.6 & 0.09 & 1 \\
            \hline
            degree\_lin & 271062.0 & 1817 & 79.38 & 1607.96 & 0.09 & 1 \\
            \hline
        \end{tabular}
        \end{adjustbox}
    \caption{Global altruism with $0.1$ altruistic constant. }
    \vspace{0.2cm}
    \end{subfigure}
    \begin{subfigure}[b]{\textwidth}
    \centering
            \setlength{\tabcolsep}{10pt} % Column separation
        \begin{adjustbox}{max width=\textwidth}
        \begin{tabular}{|c|c|c|c|c|c|c|}
            \hline
            \textbf{Initialization strategy} & \textbf{Sumcost} & \textbf{Iterations} & \textbf{SW \%} & \textbf{Iter \%} & \textbf{sum of bc at -1} & \textbf{\# of top10 at -1} \\
            \hline
            random\_2 & 509925.0 & 5223 & 100.0 & 100.0 & 0.28 & 6 \\
            \hline
            random\_5 & 509925.0 & 5330 & 100.0 & 102.05 & 0.28 & 6 \\
            \hline
            random\_1 & 860969.0 & 5293 & 59.23 & 101.34 & 0.26 & 6 \\
            \hline
            ['bc', 'Threshold', 'all from -1'] & 862924.0 & 188 & 59.09 & 3.6 & 0.27 & 6 \\
            \hline
            bc\_exp & 862970.0 & 1863 & 59.09 & 35.67 & 0.26 & 5 \\
            \hline
            degree\_exp & 862970.0 & 1865 & 59.09 & 35.71 & 0.26 & 5 \\
            \hline
            degree\_lin & 862970.0 & 4723 & 59.09 & 90.43 & 0.26 & 5 \\
            \hline
            bc\_lin & 862970.0 & 4723 & 59.09 & 90.43 & 0.26 & 5 \\
            \hline
            ['degree', 'Threshold', 'all from -1'] & 862970.0 & 4752 & 59.09 & 90.98 & 0.26 & 5 \\
            \hline
            random\_4 & 862970.0 & 5139 & 59.09 & 98.39 & 0.26 & 5 \\
            \hline
            ['bc', 'No Threshold', 'all from -1'] & 862970.0 & 5214 & 59.09 & 99.83 & 0.26 & 5 \\
            \hline
            random\_3 & 862970.0 & 5217 & 59.09 & 99.89 & 0.26 & 5 \\
            \hline
            random\_0 & 862970.0 & 5267 & 59.09 & 100.84 & 0.26 & 5 \\
            \hline
            ['degree', 'No Threshold', 'all from -1'] & 862970.0 & 8250 & 59.09 & 157.96 & 0.26 & 5 \\
            \hline
            ['bc', 'Threshold', 'all from -10'] & 6646797.0 & 49 & 7.67 & 0.94 & 0.13 & 3 \\
            \hline
            ['degree', 'Threshold', 'all from -10'] & 6646797.0 & 499 & 7.67 & 9.55 & 0.13 & 3 \\
            \hline
            ['bc', 'No Threshold', 'all from -10'] & 6646797.0 & 545 & 7.67 & 10.43 & 0.13 & 3 \\
            \hline
            ['degree', 'No Threshold', 'all from -10'] & 6646797.0 & 848 & 7.67 & 16.24 & 0.13 & 3 \\
            \hline
        \end{tabular}
        \end{adjustbox}
    \caption{Local altruism with $0.1$ altruistic constant. }
    \vspace{0.2cm}
    \end{subfigure}
    \begin{subfigure}[b]{\textwidth}
    \centering
            \setlength{\tabcolsep}{10pt} % Column separation
        \begin{adjustbox}{max width=\textwidth}
        \begin{tabular}{|c|c|c|c|c|c|c|}
            \hline
            \textbf{Initialization strategy} & \textbf{Sumcost} & \textbf{Iterations} & \textbf{SW \%} & \textbf{Iter \%} & \textbf{sum of bc at -1} & \textbf{\# of top10 at -1} \\
            \hline
            ['degree', 'Threshold', 'all from -10'] & 134905.0 & 587 & 100.0 & 100.0 & 0.14 & 2 \\
            \hline
            ['bc', 'No Threshold', 'all from -10'] & 134907.0 & 633 & 100.0 & 107.84 & 0.14 & 2 \\
            \hline
            ['bc', 'Threshold', 'all from -10'] & 135183.0 & 126 & 99.79 & 21.47 & 0.32 & 6 \\
            \hline
            ['bc', 'Threshold', 'all from -1'] & 135204.0 & 101 & 99.78 & 17.21 & 0.36 & 8 \\
            \hline
            ['degree', 'No Threshold', 'all from -10'] & 137726.0 & 251 & 97.95 & 42.76 & 0.09 & 1 \\
            \hline
            bc\_exp & 143682.0 & 134 & 93.89 & 22.83 & 0.34 & 9 \\
            \hline
            degree\_exp & 143838.0 & 128 & 93.79 & 21.81 & 0.28 & 4 \\
            \hline
            ['degree', 'Threshold', 'all from -1'] & 146730.0 & 3100 & 91.94 & 528.11 & 0.2 & 3 \\
            \hline
            ['bc', 'No Threshold', 'all from -1'] & 149540.0 & 3291 & 90.21 & 560.65 & 0.18 & 2 \\
            \hline
            degree\_lin & 149589.0 & 2273 & 90.18 & 387.22 & 0.19 & 2 \\
            \hline
            bc\_lin & 149589.0 & 2273 & 90.18 & 387.22 & 0.19 & 2 \\
            \hline
            random\_4 & 152400.0 & 2490 & 88.52 & 424.19 & 0.14 & 1 \\
            \hline
            random\_3 & 155075.0 & 2093 & 86.99 & 356.56 & 0.13 & 2 \\
            \hline
            random\_5 & 155135.0 & 2176 & 86.96 & 370.7 & 0.11 & 2 \\
            \hline
            random\_0 & 155152.0 & 2357 & 86.95 & 401.53 & 0.15 & 2 \\
            \hline
            random\_1 & 157941.0 & 1947 & 85.41 & 331.69 & 0.06 & 0 \\
            \hline
            random\_2 & 157947.0 & 2173 & 85.41 & 370.19 & 0.15 & 2 \\
            \hline
            ['degree', 'No Threshold', 'all from -1'] & 160782.0 & 5016 & 83.91 & 854.51 & 0.14 & 2 \\
            \hline
        \end{tabular}
        \end{adjustbox}
    \caption{Global altruism with $1.0$ altruistic constant. }
    \vspace{0.2cm}
    \end{subfigure}
    \begin{subfigure}[b]{\textwidth}
    \centering
            \setlength{\tabcolsep}{10pt} % Column separation
        \begin{adjustbox}{max width=\textwidth}
        \begin{tabular}{|c|c|c|c|c|c|c|}
            \hline
            \textbf{Initialization strategy} & \textbf{Sumcost} & \textbf{Iterations} & \textbf{SW \%} & \textbf{Iter \%} & \textbf{sum of bc at -1} & \textbf{\# of top10 at -1} \\
            \hline
            random\_0 & 142327.0 & 5254 & 100.0 & 100.0 & 0.35 & 8 \\
            \hline
            random\_4 & 142589.0 & 5096 & 99.82 & 96.99 & 0.35 & 8 \\
            \hline
            random\_1 & 142611.0 & 5315 & 99.8 & 101.16 & 0.34 & 7 \\
            \hline
            random\_3 & 142646.0 & 5242 & 99.78 & 99.77 & 0.34 & 6 \\
            \hline
            ['bc', 'Threshold', 'all from -10'] & 163820.0 & 121 & 86.88 & 2.3 & 0.35 & 9 \\
            \hline
            ['bc', 'Threshold', 'all from -1'] & 163958.0 & 144 & 86.81 & 2.74 & 0.34 & 8 \\
            \hline
            ['degree', 'Threshold', 'all from -10'] & 163958.0 & 571 & 86.81 & 10.87 & 0.34 & 8 \\
            \hline
            ['bc', 'No Threshold', 'all from -10'] & 163958.0 & 617 & 86.81 & 11.74 & 0.34 & 8 \\
            \hline
            ['degree', 'No Threshold', 'all from -10'] & 163958.0 & 920 & 86.81 & 17.51 & 0.34 & 8 \\
            \hline
            bc\_exp & 163958.0 & 1847 & 86.81 & 35.15 & 0.34 & 8 \\
            \hline
            degree\_lin & 163958.0 & 4727 & 86.81 & 89.97 & 0.34 & 8 \\
            \hline
            bc\_lin & 163958.0 & 4727 & 86.81 & 89.97 & 0.34 & 8 \\
            \hline
            ['degree', 'Threshold', 'all from -1'] & 163958.0 & 4742 & 86.81 & 90.26 & 0.34 & 8 \\
            \hline
            ['bc', 'No Threshold', 'all from -1'] & 163958.0 & 5204 & 86.81 & 99.05 & 0.34 & 8 \\
            \hline
            ['degree', 'No Threshold', 'all from -1'] & 163958.0 & 8252 & 86.81 & 157.06 & 0.34 & 8 \\
            \hline
            degree\_exp & 164325.0 & 1851 & 86.61 & 35.23 & 0.32 & 7 \\
            \hline
            random\_2 & 164524.0 & 5330 & 86.51 & 101.45 & 0.33 & 6 \\
            \hline
        \end{tabular}
        \end{adjustbox}
    \caption{Local altruism with $1.0$ altruistic constant. }
    \vspace{0.2cm}
    \end{subfigure}
    \caption{Attributes of strategy profiles in NE reached by various initialization strategies for the \textit{message} dataset.}
    \label{fig:college_table}
\end{figure}

\begin{figure}[!ht]
    \centering
    
    \includegraphics[height=6cm]{figures3/eu/0.1/email-Eu-core-temporal[0.1]_NE_runs_global.pdf}
     \includegraphics[height=6cm]{figures3/eu/1.0/email-Eu-core-temporal[1.0]_NE_runs_global.pdf}
    \includegraphics[height=6cm]{figures3/eu/0.1/email-Eu-core-temporal[0.1]_NE_runs_local.pdf}
   \includegraphics[height=6cm]{figures3/eu/1.0/email-Eu-core-temporal[1.0]_NE_runs_local.pdf}
    \caption{Correlation between selected attributes of NE and the achieved social cost SW, \textit{mail}, top/bottom:  global/local, left/right: $a_u=0.1$/$a_u=1.0$. For each figure, the 3 scatterplots are: convergence time, aggregated betw. centr. for max nodes, number of Top-10 users in max nodes. Results relative to best-case NE for given setting.}
    \label{fig:eu_NE_stats}
\end{figure}\clearpage

\begin{comment}
    
\begin{figure}[tb]
    \centering
    \includegraphics[width=0.9\textwidth]{figures3/eu/0.1/[email-Eu-core-temporal][All][0.1][SO]_global_table.png}
    \includegraphics[width=0.9\textwidth]{figures3/eu/0.1/[email-Eu-core-temporal][All][0.1][SO]_local_table.png}
    \includegraphics[width=0.9\textwidth]{figures3/eu/1.0/[email-Eu-core-temporal][All][1.0][SO]_global_table.png}
    \includegraphics[width=0.9\textwidth]{figures3/eu/1.0/[email-Eu-core-temporal][All][1.0][SO]_local_table.png}
    \caption{Attributes of SO runs in the \textit{mail} dataset. Tables in order: global altruism with $0.1$, local altruism with $0.1$, global altruism with $1.0$, local altruism with $1.0$.}
    \label{fig:eu_table_SO}
\end{figure}

\begin{figure}[tb]
    \centering
    \includegraphics[width=0.9\textwidth]{figures3/college/0.1/[CollegeMsg][All][0.1][SO]_global_table.png}
    \includegraphics[width=0.9\textwidth]{figures3/college/0.1/[CollegeMsg][All][0.1][SO]_local_table.png}
    \includegraphics[width=0.9\textwidth]{figures3/college/1.0/[CollegeMsg][All][1.0][SO]_global_table.png}
    \includegraphics[width=0.9\textwidth]{figures3/college/1.0/[CollegeMsg][All][1.0][SO]_local_table.png}
    \caption{Attributes of SO runs in the \textit{college} dataset. Tables in order: global altruism with $0.1$, local altruism with $0.1$, global altruism with $1.0$, local altruism with $1.0$.}
    \label{fig:college_table_SO}
\end{figure}

\end{comment}
